# Supplementary material for: Automated Repair of Ambiguous Problem Descriptions for LLM-Based Code Generation
Source: arXiv:2505.07270 source file (2025-09-24)
Supplement: Supplementary file 1 [file appendix.tex]

%% \pagebreak
\twocolumn
\appendix

\subsection{Details of Experiments}

In this section, we provide further details regarding \projName repair performance, and analyze the types of ambiguity in \changes{problem descriptions} it repairs. For each requirement, we compute the \emph{Pass@1 delta} as
\begin{equation*}
    \Delta = Pass@1_{repaired} - Pass@1_{original}.
\end{equation*}
We call a case a \emph{success} if its Pass@1 delta is greater than zero, and a \emph{failure} if the delta is less than zero.
We also record whether the semantic entropy of the prompt decreases or increases after applying our repair procedure. 
Table \ref{tab:case_study} summarizes the raw counts (over three independent runs), and Figure \ref{fig:passk_delta} visualizes the full distribution of Pass@1 deltas.

\begin{table}[ht]
  \centering
  \setlength{\tabcolsep}{1.5pt}
  \caption{Summary of \projName repairs}
  \label{tab:case_study}
  \begin{tabular}{llrrrrr}
    \toprule
    Model & Dataset   & Repairs & Success & Failure & Decreased & Increased \\
    \midrule
    \multirow{2}{*}{Deepseek}
     & HumanEval+ & 33            & 15/14/17        & 3/4/2        & 28/27/25             & 1/1/0               \\
     & MBPP+      & 73            & 21/23/22        & 9/6/7        & 60/59/58             & 1/0/1                 \\
    \midrule
    \multirow{2}{*}{Qwen2.5}
     & HumanEval+ & 34            & 11/11/14        & 5/6/1        & 23/24/24             & 1/1/1                    \\
     & MBPP+      & 64            & 20/19/22        & 4/5/2        & 40/41/41             & 3/1/2                      \\
    \midrule
    \multirow{2}{*}{GPT-4o}
     & HumanEval+ & 65            & 23/28/23        & 7/5/8        & 58/57/55             & 0/0/0                     \\
     & MBPP+      & 120            & 28/29/37        & 16/16/18        & 107/100/101             & 3/0/4                     \\
    \bottomrule
  \end{tabular}
\end{table}

\begin{figure}
    \centering
    \includegraphics[width=\columnwidth]{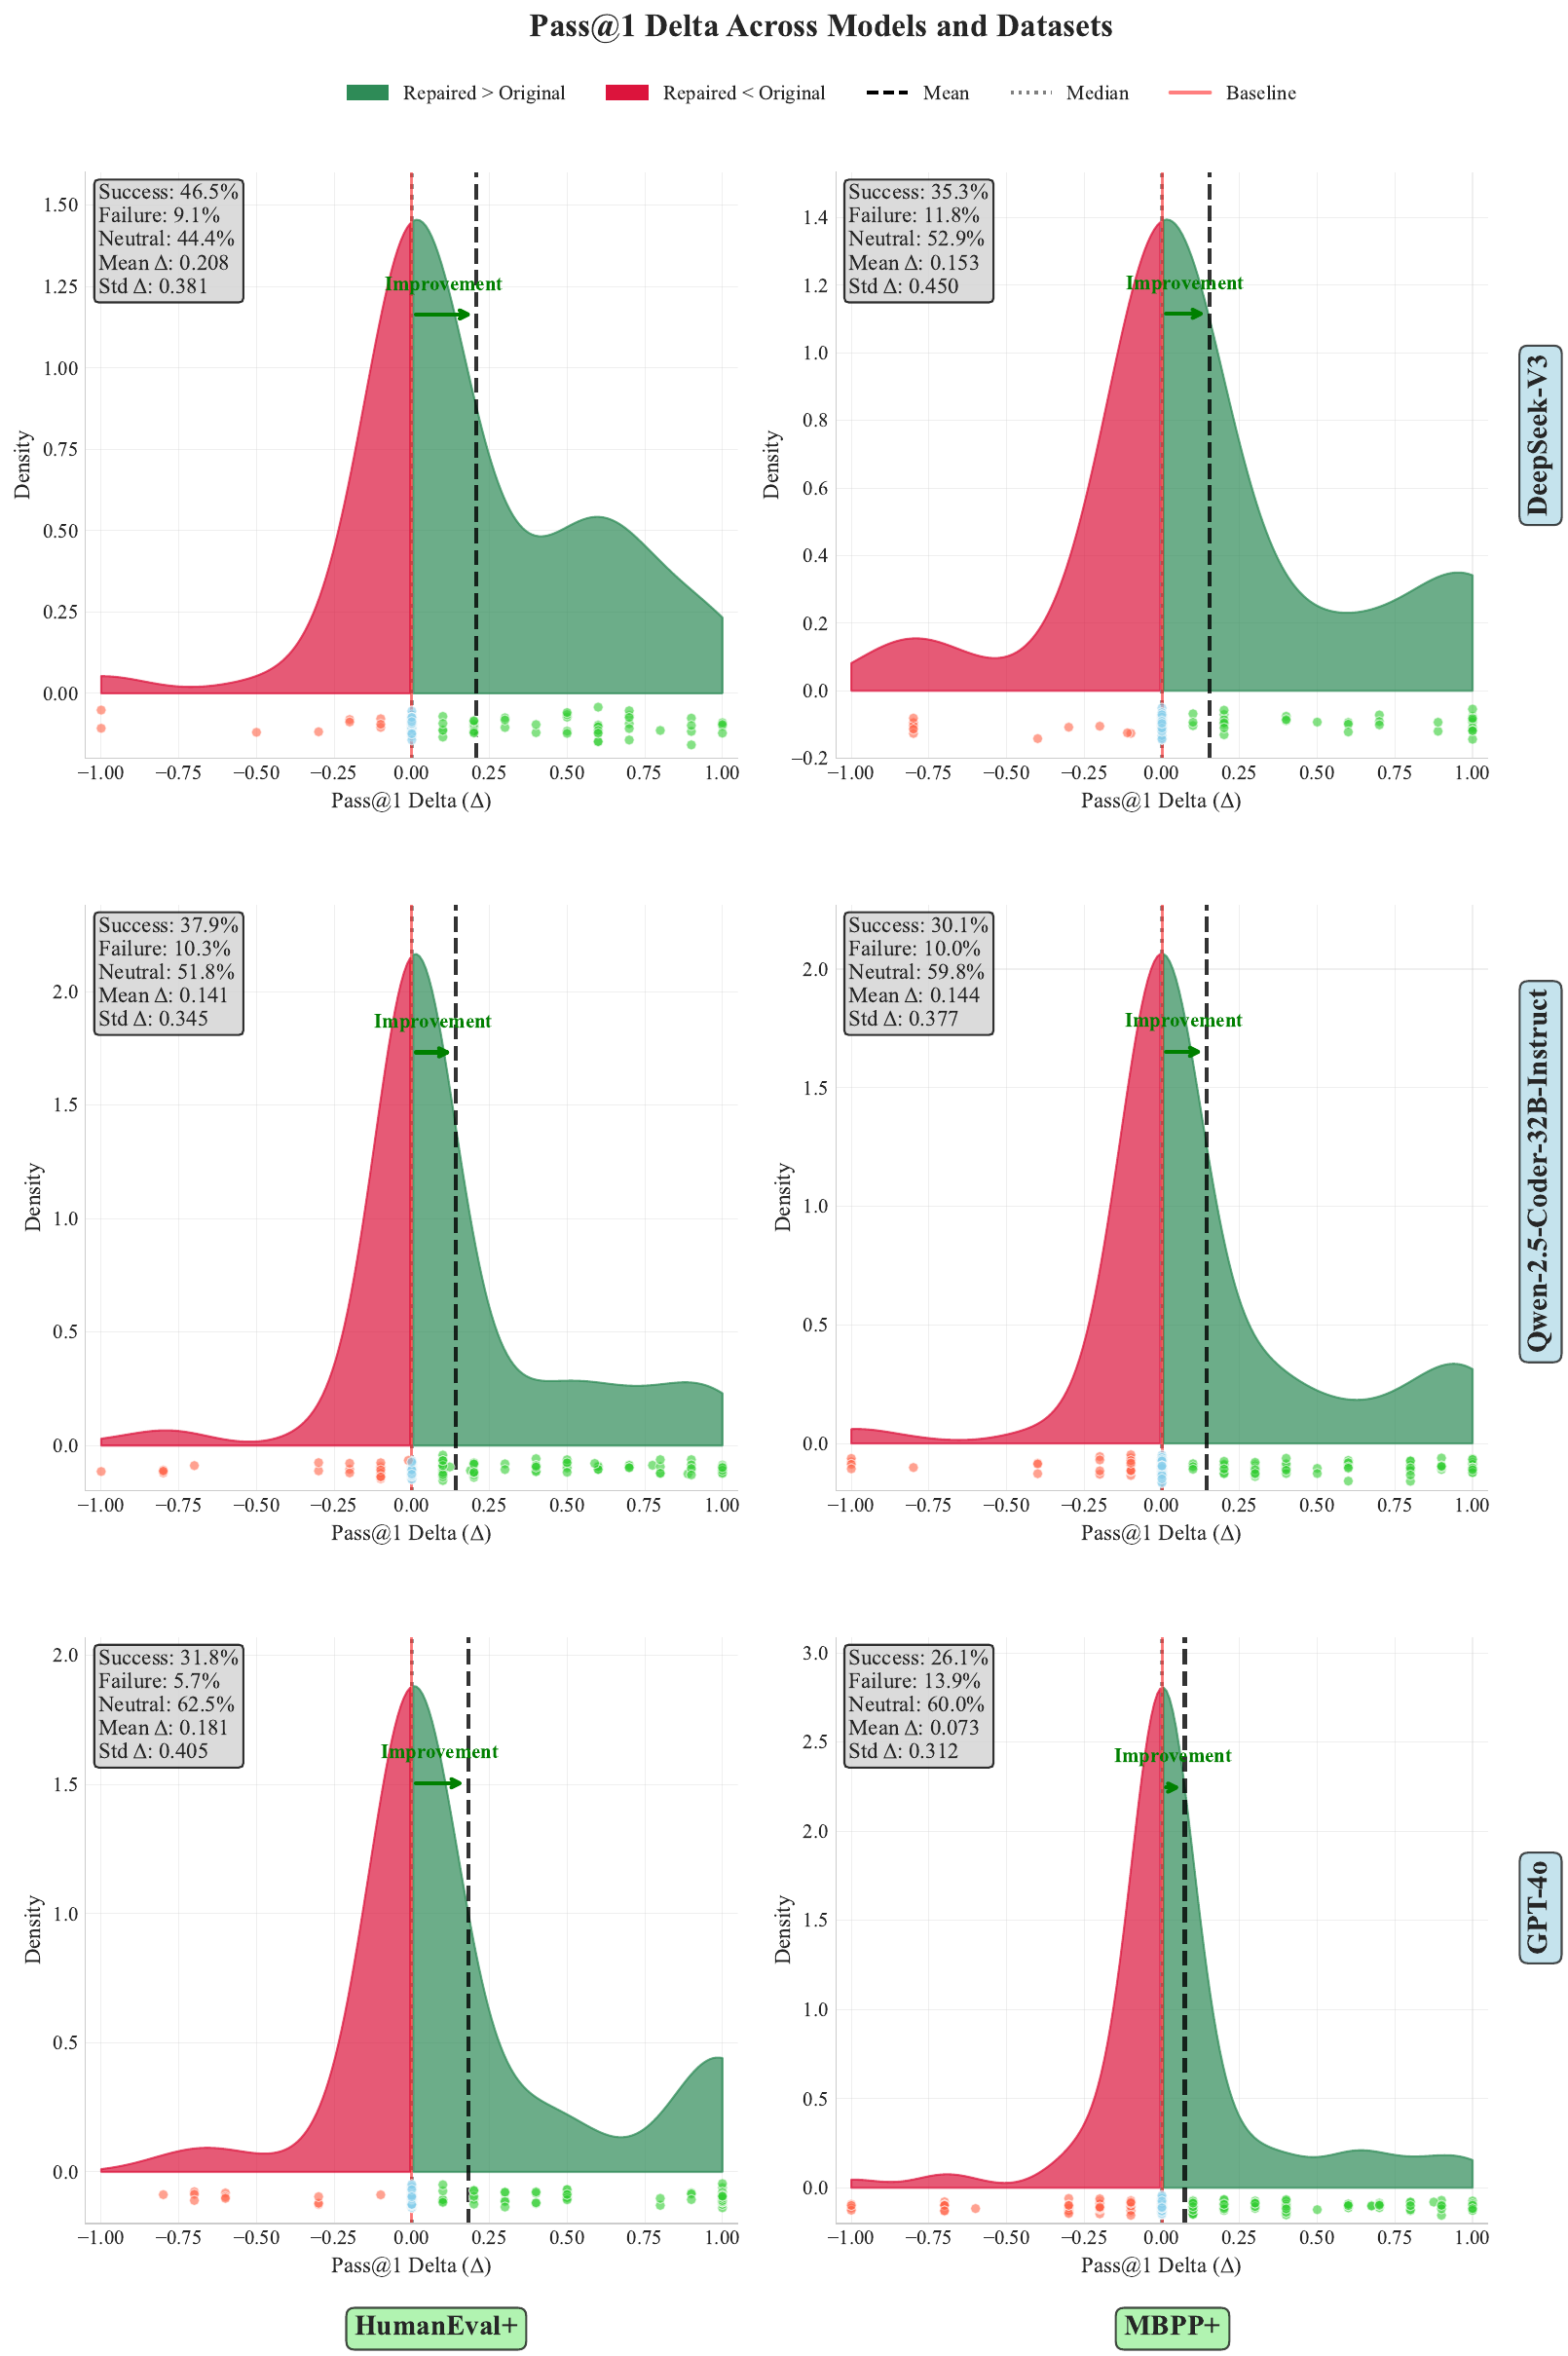}
    \caption{The distribution of Pass@1 delta on all repairs. Here, each colored curve is a Kernel Density Estimate (KDE): the green region corresponds to $\Delta>$0 (success), and the red region to $\Delta<$0 (failure). The dashed vertical line marks the mean $\Delta$ for each model–dataset pairing, and the dotted line marks the median.}
    \label{fig:passk_delta}
\end{figure}

\subsection{Case analysis}

For the successfully repaired cases, our manual inspection identified three common types of fixes: edge case repair, ambiguous phrase repair (when a phrase has two meanings) and ambiguous input/output (I/O) format repair. For each reason, we provide one illustrating example.

\paragraph{Edge case repair}
This example shows how \projName explicitly handles the scenario where the lower bound exceeds the upper bound, resolving a previously implicit edge case.

\begin{tcolorbox}[colframe=RedOrange!100, colback=gray!3, title=Ambiguous Requirement (HumanEval/102), fonttitle=\centering, before upper=\raggedright, boxrule=0.8mm, sharp corners=southwest, left=2pt, right=2pt, top=2pt, bottom=2pt, boxsep=1pt]
        \small
           This function takes two positive numbers x and y and returns the
    biggest even integer number that is in the range [x, y] inclusive. If 
    there's no such number, then the function should return -1. For example:
    \begin{lstlisting}
choose_num(12, 15) = 14
choose_num(13, 12) = -1
    \end{lstlisting}
        \end{tcolorbox}
                \begin{tcolorbox}[colframe=darkgreen!100, colback=gray!3, title=Repaired Requirement (Text Only), fonttitle=\centering, before upper=\raggedright, boxrule=0.8mm, sharp corners=southwest, left=2pt, right=2pt, top=2pt, bottom=2pt, boxsep=1pt]
        \small
           This function takes two positive integers x and y and returns the largest even integer within the range [x, y] inclusive. \hl{If x is greater than y}, or if there are no even numbers in the range, the function returns -1.
        \end{tcolorbox}

\paragraph{Ambiguous phrase repair}
In this example, the phrase “same characters” is clarified to specify that character frequency and order do not affect the check.

        \begin{tcolorbox}[colframe=RedOrange!100, colback=gray!3, title=Ambiguous Requirement (HumanEval/54), fonttitle=\centering, before upper=\raggedright, boxrule=0.8mm, sharp corners=southwest, left=2pt, right=2pt, top=2pt, bottom=2pt, boxsep=1pt]
        \small
           Check if two words have the same characters.
        \begin{lstlisting}           
>>> same_chars('eabcdzzzz', 'dddzzzzzzzddeddabc')
True
>>> same_chars('abcd', 'dddddddabc')
True
>>> same_chars('dddddddabc', 'abcd')
True
>>> same_chars('eabcd', 'dddddddabc')
False
>>> same_chars('abcd', 'dddddddabce')
False
>>> same_chars('eabcdzzzz', 'dddzzzzzzzddddabc')
False
        \end{lstlisting}           
        \end{tcolorbox}
                \begin{tcolorbox}[colframe=darkgreen!100, colback=gray!3, title=Repaired Requirement (Text Only), fonttitle=\centering, before upper=\raggedright, boxrule=0.8mm, sharp corners=southwest, left=2pt, right=2pt, top=2pt, bottom=2pt, boxsep=1pt]
        \small
           Check if two words contain exactly the same set of characters, \hl{regardless of the frequency or order of the characters}.
        \end{tcolorbox}

\paragraph{Ambiguous I/O format repair}
This example demonstrates how explicitly stating output formatting, that is excluding quotation marks—eliminates ambiguity.

        \begin{tcolorbox}[colframe=RedOrange!100, colback=gray!3, title=Ambiguous Requirement (Mbpp/563), fonttitle=\centering, before upper=\raggedright, boxrule=0.8mm, sharp corners=southwest, left=2pt, right=2pt, top=2pt, bottom=2pt, boxsep=1pt]
        \small
    Write a function to extract values between quotation marks from a string.
        \begin{lstlisting}
assert extract_values('"Python", "PHP", "Java"')==['Python', 'PHP', 'Java']
        \end{lstlisting}           
        \end{tcolorbox}
                \begin{tcolorbox}[colframe=darkgreen!100, colback=gray!3, title=Repaired Requirement (Text Only), fonttitle=\centering, before upper=\raggedright, boxrule=0.8mm, sharp corners=southwest, left=2pt, right=2pt, top=2pt, bottom=2pt, boxsep=1pt]
        \small
    Extract all substrings that are enclosed within double quotation marks from the input string.
    
    \hl{Each substring should be captured without the surrounding quotes.}
        \end{tcolorbox}

\subsection{LLM Prompts}

In this section of the Appendix, we include all prompts provided to the LLMs in \projName. Placeholders delimited by angle brackets are substituted at runtime.

\begin{promptbox}[Example Extraction Prompt]
\textbf{$<$specification$>$}

Given a programming problem description, your task is to locate and extract *all example cases* found in the description, including in-text illustrations (e.g., `for example, if...') or standalone example sections. 

An "example" should include a sample input (argument) and output (return value) pair.
\end{promptbox}

\begin{promptbox}[Test Case Generation Prompt]
\textbf{$<$specification$>$}

Given a requirement containing a function signature and docstring, your task is to generate inputs for function \textbf{$<$entry\_point$>$}  to cover all functionalities, including normal cases and corner cases.

Ensure the type and number of argument are matching the function signature. In this requirement, the argument number is \textbf{$<$para\_number$>$} .
Don't output the function name, only the test inputs. If there are multiple arguments, separate them with commas.
\end{promptbox}

\begin{promptbox}[Code Generation Prompt]

Here is the given programming problem to solve.

\textbf{$<$specification$>$}

Please implement the \textbf{$<$entry\_point$>$} function and make sure that it matches the signature and functionality described in the requirement. 
Ensure to include necessary imports for function signature and function body.
Don't output any explanation or comments, only the function implementation.
\end{promptbox}

\begin{promptbox}[Program Repair Prompt]
\textbf{$<$specification$>$}

\textbf{$<$faulty\_program$>$}

\textbf{$<$test\_inputs$>$}

\textbf{$<$actual\_outputs$>$}

\textbf{$<$expected\_outputs$>$}

Your task is to:

1. Carefully analyze the task requirement to understand the intended behavior of the faulty program.

2. Examine the provided test cases, comparing the actual output with the expected output to clearly identify the underlying issue(s) such as logic errors, incorrect calculations, edge-case mishandling, or syntax issues.

3. Fix the Python function, ensuring the revised code passes all the provided test cases by generating the correct outputs.

\end{promptbox}

\begin{promptbox}[Contrastive Specification Inference Prompt]
\textbf{$<$specification$>$}

\textbf{$<$test\_inputs$>$}

\textbf{$<$selected\_program$>$}

\textbf{$<$selected\_outputs$>$}

\textbf{$<$rejected\_programs$>$}

\textbf{$<$rejected\_outputs$>$}

Your task is to:

1. Carefully analyze the provided specification, identifying and clearly stating the specific wording or phrases that could be interpreted in multiple ways.

2. Analyze the selected program and selected outputs to determine the intended functionality and behavior.

3. Analyze the rejected implementation and rejected outputs to determine the unintended functionality and behavior.

4. State the potential sources of ambiguity that led to the divergence in outputs. 

5. Concisely revise the requirement to remove ambiguity, aligning with behaviors of selected program and diverging from behaviors of rejected programs. 
\end{promptbox}
